# Supplementary material for: MSG-BART: Multi-granularity Scene Graph-Enhanced Encoder-Decoder Language Model for Video-grounded Dialogue Generation
Source: arXiv:2311.12820 source file (2023-09-26)
Supplement: Supplementary file 1 [file 07Appendix.tex]

\appendix
\newpage
\section{Feature Extraction}
\label{sec:appendix}
%The previous method did not make effective use of the information in the video, but simply extracted the overall audio-visual features of the video, putting the main target on the text patterns. To overcome this shortcoming, 

A variety of information is mined from the video. In addition to the multi-dimensional video information, such as visual features, and audio features at different granularity, we also extract entities and spatio-temporal action information using the spatio-temporal scene graph.

\paragraph{Visual feature} The video is segmented into consecutive video frames $I_{\rm v}= \{I_{\rm v}^1, I_{\rm v}^2, \ldots, I_{\rm v}^{M}\}$ at a rate of $1$fps. Visual features $f_{\rm V}^{i}$ are then extracted from video frames of different duration by ActionCLIP image encoder ViT, which is pre-trained on the Kinetics-400 dataset \citep{kinetics-400}.
\begin{equation}
f_{\rm V}^{i} = \operatorname{ActionCLIP}(\operatorname{Concat}(I_{\rm v}^k)|_{k = n}^{n+m})
\end{equation}
where $n$ and $n+m$ denote the start and end points of the extracted video frames. The visual feature $F_V$ is obtained as ${F_{\rm V}=\operatorname{Concat}(f_{\rm V}^{1}, f_{\rm V}^{2}, \ldots, f_{\rm V}^{t})}$.

\paragraph{Audio feature}The audio is divided into audio clips $W = \{W_1, W_2, \ldots, W_{M}\}$ of the same time length according to the extraction frequency of the video frames. The pre-trained Wav2CLIP is then used to extract audio features $f_{\rm A}^{i}$ from the audio clips of different durations.
\begin{equation}
f_{\rm A}^{i} = \operatorname{Wav2CLIP}(\operatorname{Concat}(W_k)|_{k = n}^{n+m})
\end{equation}
where $n$ and $n+m$ denote the start and end point of the extracted audio clips, the audio feature $F_{\rm V}$ is represented as ${F_{\rm A}=\operatorname{Concat}(f_{\rm A}^{1}, f_{\rm A}^{2}, \ldots, f_{\rm A}^{t})}$.

\paragraph{Scene graph} A spatio-temporal scene graph is generated for each video frame based on the extracted video frames. First, entities in the frame are detected by faster R-CNN \citep{frcnn}, where the detector provides the visual feature $O_{\rm V}=\{v_1, v_2, \ldots, v_{N}\}$, the bounding box $O_{\rm B}=\{b_1, b_2, \ldots, b_{N}\}$, the object label $O_{\rm L}=\{l_1, l_2, \ldots, l_{N}\}$, and then the spatial, contact, and attention relationships between the different entities are generated using the STTran model pre-trained on the Action Genome by semi constraint.
\begin{equation}
r_{ij} = \operatorname{STTran}(v_i,b_i,l_i,v_j,b_j,l_j) \in R
\end{equation}
where $i$, $j$ denote the source node and target node, the relationship  $r_{ij}$ shows spatial, contact, and attention relationships together, and the set of relations $\varepsilon$ is defined as $\varepsilon=\{r_{ij} \}$. Thus, the spatio-temporal scene graph is defined as $\mathcal{G}=\{(x_i,r_{ij},x_j)|x_i,x_j\in\nu,r_{ij}\in \varepsilon\}$, where $\nu=\{x_1,...,x_N\}$ denotes the set of $N$ object nodes.

% In addition, the set of the relationships are shown in table~\ref{tab:relationship}

% \begin{table*}[t]
%     \centering
%     \begin{tabular}{llll}\hline
%         \textbf{attention} & \textbf{spatial} & \multicolumn{2}{c}{\textbf{contact}}  \\ \hline
%         looking at & above & carrying  & not contacting  \\ 
%         not looking at & behind & covered by  & sitting on  \\ 
%         unsure & beneath & drinking from  & standing on  \\ 
%         ~ & in & eating   & touching   \\ 
%         ~ & in front of & have it on the back  & twisting  \\ 
%         ~ & on the side of & holding   & wearing   \\ 
%         ~ & ~ & leaning on  & wiping  \\ 
%         ~ & ~ & lying on  & writing on   \\ \hline
%     \end{tabular}
%     \caption{The set of relationship}
%     \label{tab:relationship}
% \end{table*}

\section{Experimental Setup}
\label{sec:appendix-setup}
\paragraph{Training} We extracted visual and audio features by ActionCLIP and Wav2CLIP with a time duration of 4s for coarse-grained features and 1s for fine-grained features. In our experiments, we initialized our model using the weights of the BART-base\footnote{\url{https://huggingface.co/facebook/bart-base}} model, which contains 139$\rm M$ parameters. In the training phase, we used 4 heads in the multi-head attention model, the hidden size was 768 and the batch size was 32. We adopted an AdamW~\citep{Loshchilov2018} optimizer with a learning rate for fine-tuning BART of 6.25e-5 and a learning rate of 6.25e-4 for training the GVP module. 
\paragraph{Inference}During the decoding phase, we used the beam search algorithm with a beam size of 6 and a penalty factor of 0.6.

\section{Experiments with LLM}
\label{sec:appendix_llm}

\begin{table*}[t]
\centering
\setlength\tabcolsep{10pt}
\resizebox{1\linewidth}{!}
{
\begin{tabular}{lccccccccc}
\bottomrule[1pt]
\textbf{Models} & Sampling Stratege & PLM Param. & \bf B@1 &\bf B@2 &\bf B@3 &\bf B@4 &\bf MET &\bf ROU &\bf CID \\ \hline 
AVSD-LLaMA-7B & Beam Search  &7B & \textbf{0.731} & \textbf{0.599} &\textbf{0.493} &\textbf{0.408} &\textbf{0.276} &\textbf{0.570} &\textbf{1.064} \\
AVSD-LLaMA-7B& Greedy Search &7B & 0.685& 0.550& 0.446& 0.366& 0.245& 0.537& 0.944 \\ 
MSG-BART (Ours) & Beam Search   &139M & 0.719   & 0.581   & 0.473  & 0.390   & 0.268   & 0.556    & 1.008  \\ 
\hline
\end{tabular}
}
\caption{Evaluation result of AVSD-LLaMA-7B on DSTC10-AVSD official test set with different sampling strategies}
\label{tab:table-llm}

\end{table*}
\paragraph{Analysis} We also conduct the experiments of large language models on DSTC10-AVSD official test set and the results are shown in Table~\ref{tab:table-llm}.
It can be seen that our model outperforms the AVSD-LLaMA-7B with greedy search. Though the greedy search is the general sampling strategy in the real-world application of the large language models, it cannot truly demonstrate that the MSG-BART outperforms AVSD-LLaMA-7B. Considering the model size difference of 50 times, it can indicate the superiority of our model in a certain sense. Furthermore, the AVSD-LLaMA-7B with beam search yields the most performance gains than the others. Due to the computational resources, we cannot adapt our method to a large language model to prove the advantage of our method, which consists of multi-granularity scene graphs, the GVP module, and the multi-pointer network, and compare these in a fair situation.
In the future, we will do more experiments with a larger language model than BART-base to prove the effectiveness of our method, such as T5-large (738M) and T5-xl (3B).
\paragraph{Experimental Setup} For AVSD-LLaMA-7B, we concatenated the visual feature and audio feature in the time dimension as the video feature and transfer their dimension to 768 by using two separate projection linear layers. Then, we concatenated the video feature, dialogue history, and question as the input into the LLaMA-7B\footnote{\url{https://huggingface.co/decapoda-research/llama-7b-hf}}, which was fine-tuned using Low-Rank Adaptation \citep{hu2022lora} to acquire the video-grounded answer. We adopted an AdamW optimizer with a learning rate of 1e-4 and only unfroze the projection linear layers and LoRA weights. %Considering the computing cost and application scenarios, we adopt the general sampling strategy in large language models during the decoding phase, which is the greedy search algorithm.
During the decoding phase, we adopt the greedy search algorithm and beam search algorithm with the same setting as MSG-BART.
